# Supplementary material for: A Trade-Off Between Path Entanglement and Quantum Sensitivity
Source: arXiv:2411.18832 ancillary file (2025-04-25)
Supplement: Supplementary file 1 [file tradeoff_supp.pdf]

# Supplementary Information for “A Trade-Off Between Path Entanglement and Quantum Sensitivity”

Benjamin Lou,<sup>1,\*</sup> Hudson A. Loughlin,<sup>1</sup> and Nergis Mavalvala<sup>1</sup>

<sup>1</sup>*LIGO Laboratory, Massachusetts Institute of Technology, Cambridge, MA 02139*

(Dated: April 25, 2025)

## I. DETAILS ON THE SETUP AND QFI CALCULATIONS

An  $N$ -mode bosonic system is described by  $N$  pairs of canonically conjugate operators [1, 2]

$$\hat{\mathbf{q}} = (\hat{x}_1, \hat{p}_1, \dots, \hat{x}_N, \hat{p}_N)^T = (\hat{q}_1, \dots, \hat{q}_{2N})^T. \quad (1)$$

Setting  $\hbar = 2$ , the canonical commutation relations are  $[\hat{q}_j, \hat{q}_k] = 2i\Omega_{jk}$ , where  $\Omega$  is the matrix of the symplectic form:

$$\Omega := \begin{bmatrix} \omega & & \\ & \ddots & \\ & & \omega \end{bmatrix} \quad \omega := \begin{bmatrix} 0 & 1 \\ -1 & 0 \end{bmatrix}. \quad (2)$$

We assume the state is zero-mean, meaning  $\langle \hat{q}_i \rangle = 0$ .

We are interested in the sensitivity of measuring small phase shifts on a zero-mean Gaussian state with covariance matrix  $\mathbf{V}(0)$ . Define the generator

$$\mathbf{g} = \begin{bmatrix} g_1 \omega & & \\ & \ddots & \\ & & g_N \omega \end{bmatrix}. \quad (3)$$

Here,  $g_a \in \mathbb{R}$  for  $a = 1, \dots, N$ . Then,

$$\mathbf{V}(\phi) = e^{\phi \mathbf{g}} \mathbf{V}(0) e^{-\phi \mathbf{g}} \quad (4)$$

is the covariance matrix of the state after a phase shift of magnitude  $g_a \phi$  for each mode  $a$ .

The QFI of a pure, zero-mean Gaussian state at  $\phi = \phi_0$  is given by [3–5]

$$H = \frac{1}{4} \text{Tr} \left( \mathbf{V}^{-1} \mathbf{V}' \mathbf{V}^{-1} \mathbf{V}' \right), \quad (5)$$

where the matrices are evaluated at  $\phi = \phi_0$ , and  $\mathbf{V}' = \partial_\phi \mathbf{V}$ . By differentiating eq. (4), we find

$$\mathbf{V}' = [\mathbf{g}, \mathbf{V}], \quad (6)$$

which allows us to expand eq. (5) into

$$\frac{1}{2} \text{Tr} \left( \mathbf{g}^2 - \mathbf{V} \mathbf{g} \mathbf{V}^{-1} \mathbf{g} \right). \quad (7)$$

Since  $\mathbf{g}$  commutes with  $e^{\phi_0 \mathbf{g}}$ , this expression is independent of  $\phi_0$ , so we can take  $\mathbf{V} = \mathbf{V}(0)$  in this formula. To handle  $\mathbf{V}^{-1}$ , note that since the state is pure,  $\mathbf{V}$  is symmetric and symplectic by Proposition 2 in section II below. Therefore,  $\mathbf{V} \Omega \mathbf{V} = \Omega$ , and since  $\Omega^{-1} = -\Omega$ , this implies

$$\mathbf{V}^{-1} = -\Omega \mathbf{V} \Omega. \quad (8)$$

---

\* [benlou5@mit.edu](mailto:benlou5@mit.edu)

Defining

$$\begin{aligned}\mathbf{G} &:= \text{diag}(g_1, g_1, g_2, g_2, \dots, g_N, g_N) \\ &= -\mathbf{\Omega}\mathbf{g},\end{aligned}\tag{9}$$

we find that eq. (7) becomes the desired

$$H = \frac{\text{Tr} \left( (\mathbf{V}\mathbf{G})^2 - \mathbf{G}^2 \right)}{2}.\tag{10}$$

We derived this for pure states, but for mixed states, the RHS is instead an upper bound. To see this, note that we can purify the mixed state into a pure, zero-mean Gaussian state by adding some extra modes [6], and we may assume these modes do not receive phase shifts. This can only increase the QFI since all measurements that could be performed before the addition can still be performed simply by ignoring the extra modes. However, the addition does not change the RHS of eq. (10) since  $\mathbf{G}$  vanishes on the extra modes, yielding the upper bound.

It is useful to express eq. (10) in terms of the blocks of  $\mathbf{V}$ . Given any  $2N \times 2N$  matrix  $\mathbf{M}$ , we write  $\mathbf{M}_{(a,b)}$  for the  $2 \times 2$  submatrix

$$\mathbf{M}_{(a,b)} = \begin{bmatrix} M_{2a-1,2b-1} & M_{2a-1,2b} \\ M_{2a,2b-1} & M_{2a,2b} \end{bmatrix}.\tag{11}$$

Now, since  $\mathbf{G}$  is diagonal, we have

$$\begin{aligned}\text{Tr} \left( (\mathbf{V}\mathbf{G})^2 \right) &= \sum_{a,b} \text{Tr}(\mathbf{V}_{(a,b)} \mathbf{G}_{(b,b)} \mathbf{V}_{(b,a)} \mathbf{G}_{(a,a)}) \\ &= \sum_{a,b} g_a g_b \text{Tr}(\mathbf{V}_{(a,b)} \mathbf{V}_{(b,a)}) \\ &= \sum_{a,b} g_a g_b \|\mathbf{V}_{(a,b)}\|^2.\end{aligned}\tag{12}$$

In the last equality, we used that  $\mathbf{V}_{(a,b)} = \mathbf{V}_{(b,a)}^T$  since  $\mathbf{V}$  is symmetric. We can now express eq. (10) as

$$H = \frac{1}{2} \sum_{a,b} g_a g_b \|\mathbf{V}_{(a,b)}\|^2 - \sum_a g_a^2.\tag{13}$$

For example, setting  $g_1 = 1$ ,  $g_a = 0$  for  $a > 1$ , we recover

$$H = \frac{\|\mathbf{V}_1\|^2}{2} - 1.\tag{14}$$

In the two-mode case, we may rewrite eq. (13) as:

$$H = \frac{g_1^2(\|\mathbf{V}_{(1,1)}\|^2 - 2) + g_2^2(\|\mathbf{V}_{(2,2)}\|^2 - 2)}{2} + g_1 g_2 \|\mathbf{V}_{(1,2)}\|^2\tag{15}$$

Next, setting  $g_1 = g_2 = 1$  in eq. (13), we have

$$H_{\text{com}} = \frac{\|\mathbf{V}_{(1,1)}\|^2 + \|\mathbf{V}_{(2,2)}\|^2 + 2\|\mathbf{V}_{(1,2)}\|^2}{2} - 2.\tag{16}$$

Using this to eliminate  $\|\mathbf{V}_{(1,2)}\|$ , eq. (15) becomes

$$H = \left( g_1^2 - g_1 g_2 \right) H_1 + \left( g_2^2 - g_1 g_2 \right) H_2 + g_1 g_2 H_{\text{com}},\tag{17}$$

where  $H_a = \|\mathbf{V}_{(a,a)}\|^2/2 - 1$  is the QFI with  $g_a = 1$ ,  $g_{b \neq a} = 0$ .

In the  $N$ -mode case with general  $g_a$ , we can similarly eliminate  $\mathbf{V}_{(a,b)}$  for  $a \neq b$  using the QFI  $H_{\text{com};(a,b)}$  from  $g_a = g_b = 1$ ,  $g_{c \neq a,b} = 0$ . This decomposes the QFI into the sum of terms corresponding to the QFI of a single phase shift and terms corresponding to the QFI of a common phase shift between any two of the modes:

$$H = \sum_a g_a \left( g_a - \sum_{b \neq a} g_b \right) H_a + \sum_{a,b \text{ with } a < b} g_a g_b H_{\text{com};a,b} \quad (18)$$

However, each common phase shift term will no longer be independent of  $\mathbf{K}$ , instead also capturing a sense of entanglement between the two modes and the rest of the system. Furthermore, we cannot derive a version of eq. (11) in the main text because the purities  $\mu_a$  from tracing out all but the  $a^{\text{th}}$  mode will no longer be the same. In other words, with  $N$  modes and an arbitrary generator, there are too many relevant notions of entanglement to allow for simple formulas. This essentially boils down to the difficulty of precisely defining multipartite entanglement [7].

## II. WILLIAMSON AND EULER DECOMPOSITIONS AND PURE STATES

Given a positive definite matrix  $\mathbf{V}$ , the Williamson decomposition says that

$$\mathbf{V} = \mathbf{S} \mathbf{V}_{\text{th}} \mathbf{S}^T, \quad (19)$$

where  $\mathbf{V}_{\text{th}} = \text{diag}(\kappa_1, \kappa_1, \kappa_2, \kappa_2, \dots, \kappa_n, \kappa_n)$  is the covariance matrix of a thermal state [1], and  $\mathbf{S}$  is a symplectic matrix, meaning it preserves the symplectic form by satisfying  $\mathbf{S} \mathbf{\Omega} \mathbf{S}^T = \mathbf{\Omega}$  ( $\mathbf{\Omega}$  is defined in eq. (2)). The  $\kappa_a$  are called the symplectic eigenvalues of  $\mathbf{V}$ . For an elegant proof, see [8].

Now, for convenience, we say that  $\mathbf{V}$  is pure when its associated zero-mean Gaussian state is pure.

**Proposition 2.** *The following are equivalent:*

1.  $\mathbf{V}$  is pure.
2.  $\det(\mathbf{V}) = 1$ .
3. The symplectic eigenvalues of  $\mathbf{V}$  are all 1.
4.  $\mathbf{V}$  is symplectic.
5. The zero-mean Gaussian state with covariance matrix  $\mathbf{V}$  is the unique zero-mean quantum state with covariance matrix  $\mathbf{V}$ .

Note that if one uses the  $\hbar = 1$  convention as in [2, 9, 10], then conditions 2-4 will need to be modified by suitable factors of  $1/2$ .

*Proof of Proposition 2.* We know that  $\mathbf{V}$  is pure exactly when the associated Gaussian state has purity  $\mu = 1$ . By [9],  $\det(\mathbf{V}) = 1/\mu^2$ , proving (1)  $\iff$  (2). Every symplectic matrix satisfies  $\det(\mathbf{S}) = 1$  (page 480 [10]), so (4)  $\implies$  (2), and thus, by eq. (19),  $\det(\mathbf{V}) = \det(\mathbf{V}_{\text{th}}) = \prod_a \kappa_a^2$ , so (3)  $\implies$  (2).

Conversely, the generalized uncertainty principle yields  $\kappa_a \geq 1$  [2, 10], so (2)  $\implies$  (3). Note that this is equivalent to  $\mathbf{V}_{\text{th}} + i\mathbf{\Omega} \geq 0$ , whereas often, the generalized uncertainty principle is stated as  $\mathbf{V} + i\mathbf{\Omega} \geq 0$ . These statements of the generalized uncertainty principle are equivalent since

$$\mathbf{V}_{\text{th}} + i\mathbf{\Omega} = \mathbf{S}^{-1}(\mathbf{V} + i\mathbf{\Omega})(\mathbf{S}^{-1})^T, \quad (20)$$

where we used that  $\mathbf{S}^{-1}$  is symplectic since the symplectic matrices form a group.

Next, (3) implies  $\mathbf{V}_{\text{th}} = \mathbf{I}$ , reducing eq. (19) to  $\mathbf{V} = \mathbf{S} \mathbf{S}^T$ . The symplectic group is closed under the transpose, since inverting  $\mathbf{S}^{-1} \mathbf{\Omega} (\mathbf{S}^{-1})^T = \mathbf{\Omega}$  yields  $\mathbf{S}^T \mathbf{\Omega}^{-1} \mathbf{S} = \mathbf{\Omega}^{-1}$ , and  $\mathbf{\Omega}^{-1} = -\mathbf{\Omega}$ . So  $\mathbf{V}$  is the product of two symplectic matrices, meaning (3)  $\implies$  (4).

So far, we have proven the equivalence of the first four statements. Notice that (5) is true when  $\mathbf{V} = \mathbf{I}$ , since a zero-mean state with identity covariance matrix has vanishing mean photon number and therefore must be the vacuum. If (3) is true, then after the symplectic transformation  $\mathbf{S}^{-1}$ , the covariance matrix is  $\mathbf{V}_{\text{th}} = \mathbf{I}$ , so the resulting state is the vacuum. Reversing the transformations implies that the original state was Gaussian, proving (3)  $\implies$  (5).

Conversely, we prove that if (3) is false, (5) is false (in fact, infinitely far off). If  $\kappa_a > 1$  for some  $a$ , it suffices to prove that the number of zero-mean states with covariance matrix  $\mathbf{V}_{\text{th}}$  is infinite, since we can transform any of these into having the desired  $\mathbf{V}$ . Since  $\mathbf{V}_{\text{th}}$  is diagonal, it then suffices to prove the infiniteness in the 1-mode case, where  $\mathbf{V}_{\text{th}} = \kappa \mathbf{I}$  with  $\kappa > 1$ . We can achieve this covariance matrix by perturbing the vacuum as  $c_1 |0\rangle + c_2 |j\rangle$ , where  $|j\rangle$  is the number state with  $j$  photons; for any  $j$  large enough, it is straightforward to verify that there will be constants  $c_1$  and  $c_2$  yielding a zero-mean state with covariance matrix  $\kappa \mathbf{I}$ .  $\square$

Note that (3)  $\implies$  (5) is a formal way of saying that minimum uncertainty states are Gaussian. Also, instead of referring to pure, zero-mean Gaussian states throughout the paper, we now see we could have referred to zero-mean states with a pure  $\mathbf{V}$ , yielding another way of motivating the states we are primarily considering.

We can further decompose the Williamson decomposition: the Euler decomposition says that any symplectic matrix  $\mathbf{S}$  can be written as

$$\mathbf{S} = \mathbf{K}_1 \mathbf{S}(\mathbf{r}) \mathbf{K}_2, \quad (21)$$

where  $\mathbf{K}_1$  and  $\mathbf{K}_2$  are symplectic orthogonal and  $\mathbf{S}(\mathbf{r}) = \text{diag}(e^{-r_1}, e^{r_1}, \dots, e^{-r_N}, e^{r_N})$  [1, 10]. Combining this with the above proposition,  $\mathbf{V} = \mathbf{S} \mathbf{S}^T = \mathbf{K}_1 \mathbf{S}(\mathbf{r})^2 \mathbf{K}_1^{-1}$ , so taking  $\mathbf{V}_{\text{in}} = \mathbf{S}(\mathbf{r})^2$  proves that any pure state's covariance matrix,  $\mathbf{V}$ , can be decomposed as

$$\mathbf{V} = \mathbf{K} \mathbf{V}_{\text{in}} \mathbf{K}^{-1}. \quad (22)$$

### III. PROOF OF THE OPTIMAL QFI THEOREM

We prove Theorem 1 and associated claims.

#### A. Proof of Proposition 1: Characterizing Unentangled Gaussian States

Recall that  $\mathbf{V}$  is decoupled if all covariances between different modes vanish. We now prove Proposition 1, restated here for convenience.

**Proposition 1.**  *$\mathbf{V} = \mathbf{K} \mathbf{V}_{\text{in}} \mathbf{K}^{-1}$  is decoupled if and only if the state is a tensor product of squeezed states with  $\mathbf{V}_{\text{in}}$ 's input squeezing levels,  $r_1 \dots r_N$ , in some order and orientation.*

This proposition is important to understanding Theorem 1, because it implies that the decoupled condition indeed signals a lack of entanglement between the modes.

We prove the proposition through a more general result that will also be useful later. Specifically, for zero-mean Gaussian states, we claim there is no entanglement between modes with vanishing covariance. More precisely, we claim that if  $\mathbf{V}$  is block-diagonal with arbitrary blocks  $\mathbf{V}_m$ , then the state decomposes as the tensor product of zero-mean Gaussian states with the  $\mathbf{V}_m$  as covariance matrices. Moreover, if the state is pure, so are the  $\mathbf{V}_m$ .

It is useful to introduce the notation that for a pure  $\mathbf{V}$ , the associated zero-mean state is  $|\mathbf{V}\rangle$ ; Proposition 2 implies that  $|\mathbf{V}\rangle$  is well-defined and Gaussian. Our claim becomes

$$\mathbf{V} = \bigoplus_m \mathbf{V}_m \implies |\mathbf{V}\rangle = \bigotimes_m |\mathbf{V}_m\rangle. \quad (23)$$

*Proof.* We have

$$\det(\mathbf{V}_m) \geq 1. \quad (24)$$

To see this, if the purity of the reduced state is  $\mu_m$ , recall  $\det(\mathbf{V}_m) = 1/\mu_m^2$ , and  $\mu_m \leq 1$ . Next, using Proposition 2, we also have

$$\prod_m \det(\mathbf{V}_m) = \det(\mathbf{V}) = 1. \quad (25)$$

Therefore,  $\det(\mathbf{V}_m) = 1$ , meaning  $|\mathbf{V}_m\rangle$  exists by Proposition 2. Then  $\bigotimes_m |\mathbf{V}_m\rangle$  is a zero-mean state that has covariance matrix  $\mathbf{V}$ , so it must be  $|\mathbf{V}\rangle$ .  $\square$

We can now quickly prove Proposition 1:

*Proof.* If  $\mathbf{V}$  is decoupled, then  $\mathbf{V} = \bigoplus_a \mathbf{V}_a$ , with each  $\mathbf{V}_a$  being  $2 \times 2$ . Then the  $|\mathbf{V}_a\rangle$  in eq. (23) are all pure, 1-mode Gaussian states, which are by definition squeezed states. The claim about the squeezing levels follows from the fact that the eigenvalues of  $\mathbf{V}$  are the union of the eigenvalues of the  $\mathbf{V}_a$ . The converse is easy since the tensor product clearly precludes correlations across modes.  $\square$

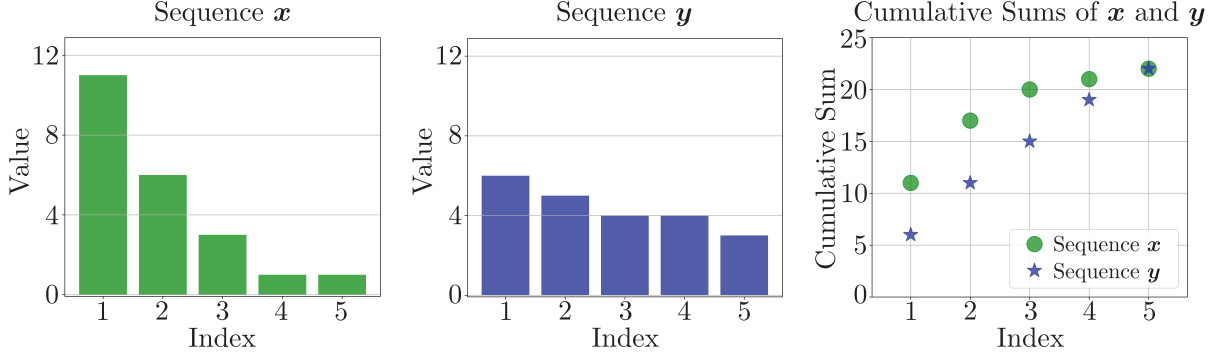

FIG. 1. Plots of the sequences  $\mathbf{x} = \{11, 6, 3, 1, 1\}$  and  $\mathbf{y} = \{6, 5, 4, 4, 3\}$ , and their cumulative sums  $\sum_{a=1}^m x_a$  and  $\sum_{a=1}^m y_a$ . We have  $\mathbf{x} \succ \mathbf{y}$ , reflecting the fact that the cumulative sums of  $\mathbf{x}$  are always at least as much as the associated ones of  $\mathbf{y}$ , while the total sums of the two sequences are the same. Intuitively,  $\mathbf{x} \succ \mathbf{y}$  because the elements of  $\mathbf{x}$  are closer to its mean.

### B. Proof of Photon Majorization Result

A key step in the proof of Theorem 1 involves using majorization to bound the mean photon numbers of each mode of a state constructed via a passive transformation on decoupled, zero-mean states. We begin with a brief overview of majorization. Majorization has found uses in subjects ranging from economics to quantum information science [11–14].

**Definition 1** (Majorization). *Given two sequences  $\mathbf{x} = \{x_a\}_{a=1}^N$  and  $\mathbf{y} = \{y_a\}_{a=1}^N$ , let  $\mathbf{x}^\downarrow = \{x_i^\downarrow\}_{i=1}^N$  denote  $\mathbf{x}$  written in nonincreasing order, and similarly for  $\mathbf{y}^\downarrow$ . We say that  $\mathbf{x}$  majorizes  $\mathbf{y}$ , written  $\mathbf{x} \succ \mathbf{y}$ , if for all  $m < N$ ,*

$$\sum_{a=1}^m x_a^\downarrow \geq \sum_{a=1}^m y_a^\downarrow \quad (26)$$

and

$$\sum_{a=1}^N x_a = \sum_{a=1}^N y_a. \quad (27)$$

Intuitively, if  $\mathbf{x} \succ \mathbf{y}$ , then  $\mathbf{y}$  looks like an averaged version of  $\mathbf{x}$ . This is illustrated in fig. 1, which plots two sequences  $\mathbf{x}$  and  $\mathbf{y}$ , with  $\mathbf{x}$  majorizing  $\mathbf{y}$ .

**Proposition 3.** *Start with an  $N$ -mode, zero-mean state (not necessarily pure or Gaussian) with a decoupled covariance matrix. Let  $\mathbf{n}_{in} = \{n_{in,a}\}_{a=1}^N$  be the mean photon numbers in each mode. Mean photon numbers of  $\mathbf{n}_{tar} = \{n_{tar,a}\}_{a=1}^N$  are possible after some passive transformation if and only if*

$$\mathbf{n}_{in} \succ \mathbf{n}_{tar}. \quad (28)$$

The proposition formalizes the intuition that passive transformations average out mean photon numbers. We note that the result can be thought of as an extension of the inability to distill entanglement from Gaussian states using Gaussian operations and classical communication [15–17]. The zero-mean condition is important; if we allow displacement in the initial states, passive transformations can siphon the displacement across all modes into one, violating the result.

We now prove the proposition. Let the original, decoupled covariance matrix be  $\mathbf{V}_{in}$ . Note that we are proving a general theorem, so  $\mathbf{V}_{in}$  need not be as it was defined in eq. (2) in the main text. However, it should be decoupled in that the covariances between different modes vanish. Suppose  $\mathbf{K}$  characterizes the passive transformation we apply to  $\mathbf{V}_{in}$ , leading to the transformed covariance matrix  $\mathbf{V} = \mathbf{K}\mathbf{V}_{in}\mathbf{K}^{-1}$ .

Instead of the  $2N \times 2N$  symplectic orthogonal matrix  $\mathbf{K}$ , it will be easier to work with its corresponding  $N \times N$  unitary matrix  $\mathbf{U}$  [2]. We state the correspondence using the  $2 \times 2$  block notation eq. (11): because  $\mathbf{K}$  commutes with the symplectic form  $\mathbf{\Omega}$  from eq. (2), each block of  $\mathbf{K}$  must take the form

$$\mathbf{K}_{(a,b)} = \begin{bmatrix} \text{Re}(U_{ab}) & \text{Im}(U_{ab}) \\ -\text{Im}(U_{ab}) & \text{Re}(U_{ab}) \end{bmatrix}, \quad (29)$$

where each  $U_{ab}$  is a complex number. It then follows from the orthogonality of  $\mathbf{K}$  that the  $U_{ab}$  must be the entries of a unitary matrix  $\mathbf{U}$ . (Physically, this correspondence means that in the Heisenberg picture, the passive transformation can be written as either  $\hat{\mathbf{a}} \mapsto \mathbf{U}\hat{\mathbf{a}}$ , where  $\hat{\mathbf{a}} = (a_1, \dots, a_N)^T$  is the vector of lowering operators, or  $\hat{\mathbf{q}} \mapsto \mathbf{K}\hat{\mathbf{q}}$ .)

Next, define a **doubly stochastic matrix** to be a square matrix with nonnegative entries such that each of its rows and columns sums to 1. Let  $\mathbf{D}$  be the matrix whose entries satisfy  $D_{ab} = |U_{ab}|^2$ . Since  $\mathbf{U}$  is unitary,  $\mathbf{U}\mathbf{U}^\dagger = \mathbf{U}^\dagger\mathbf{U} = \mathbf{I}$ , from which one deduces that  $\mathbf{D}$  is doubly stochastic.

The following fundamental theorem characterizes majorization in terms of doubly stochastic matrices (see [11] pg. 575, [12] pg.14, or [13] pg.33):

**Theorem 2** (Hardy, Littlewood, Polya). *Two sequences  $\mathbf{x}, \mathbf{y}$  satisfy  $\mathbf{x} \succ \mathbf{y}$  if and only if there exists a doubly stochastic matrix  $\mathbf{D}$  such that  $\mathbf{D}\mathbf{x} = \mathbf{y}$ .*

Using this, the following lemma suffices to prove Proposition 3:

**Lemma 1.**  $\mathbf{D}\mathbf{n}_{in} = \mathbf{n}_{tar}$ .

*Proof.* Letting  $\mathbf{2}$  be the vector containing all 2s of length  $N$ , we see that  $\mathbf{D}\mathbf{2} = \mathbf{2}$ . So the lemma is equivalent to  $\mathbf{D}(4\mathbf{n}_{in} + \mathbf{2}) = 4\mathbf{n}_{tar} + \mathbf{2}$ . This is useful because

$$\begin{aligned} 4\mathbf{n}_{in} + \mathbf{2} &= \{\text{Tr}((\mathbf{V}_{in})_{(a,a)})\}_{a=1}^N, \\ 4\mathbf{n}_{tar} + \mathbf{2} &= \{\text{Tr}(\mathbf{V}_{(a,a)})\}_{a=1}^N. \end{aligned} \quad (30)$$

Now we can prove the lemma directly:

$$\begin{aligned} \text{Tr}(\mathbf{V}_{(a,a)}) &= \text{Tr}\left(\sum_{b=1}^N \mathbf{K}_{(a,b)} (\mathbf{V}_{in})_{(b,b)} (\mathbf{K}^{-1})_{(b,a)}\right) \\ &= \sum_{b=1}^N \text{Tr}\left(\mathbf{K}_{(a,b)} (\mathbf{V}_{in})_{(b,b)} (\mathbf{K}_{(a,b)})^{-1}\right) \\ &= \sum_{b=1}^N |U_{ab}|^2 \text{Tr}((\mathbf{V}_{in})_{(b,b)}) \\ &= \sum_{b=1}^N D_{ab} \text{Tr}((\mathbf{V}_{in})_{(b,b)}). \end{aligned} \quad (31)$$

□

### C. An Inequality from Majorization

We prove a result that will help translate the majorization result of the previous section to a bound on the QFI.

**Lemma 2.** *Let  $\{c_a\}_{a=1}^N$  be a nonincreasing sequence. Suppose  $\mathbf{n} = \{n_a\}_{a=1}^N$  and  $\tilde{\mathbf{n}} = \{\tilde{n}_a\}_{a=1}^N$  are arbitrary sequences with  $\mathbf{n}$  nonincreasing. If  $\mathbf{n} \succ \tilde{\mathbf{n}}$ , then*

$$\sum_{a=1}^N c_a n_a \geq \sum_{a=1}^N c_a \tilde{n}_a. \quad (32)$$

Intuitively, averaging out the  $\mathbf{n}$  can only prevent us from taking advantage of the larger  $c_a$ .

We now prove the lemma. Some technical issues arise because the  $c_a$  may not be distinct; let us define  $\{A_m\}_{m=1}^M$  with  $A_m$  as the  $m$ th largest number among the set of  $c_a$ . In particular, the  $A_m$  are all distinct. We also define  $a(m)$  to be the largest  $a$  for which  $c_a = A_m$ .

For any sequence  $\mathbf{x} = \{x_a\}_{a=1}^N$  and integer  $a = 1, \dots, N$ , further define  $s_a(\mathbf{x}) := \sum_{b=1}^a x_b^\downarrow$ . With this notation, Definition 1 of  $\mathbf{x} \succ \mathbf{y}$  can be written as  $s_a(\mathbf{x}) \geq s_a(\mathbf{y})$  for  $a < N$  and  $s_N(\mathbf{x}) = s_N(\mathbf{y})$ .

We have

$$\sum_{a=1}^N c_a n_a = \sum_{m=1}^M (A_m - A_{m+1}) s_{a(m)}(\mathbf{n}), \quad (33)$$

where we defined  $A_{M+1} := 0$ . In particular,

$$\sum_{a=1}^N c_a (n_a - \tilde{n}_a) = \sum_{m=1}^M (A_m - A_{m+1}) (s_{a(m)}(\mathbf{n}) - s_{a(m)}(\tilde{\mathbf{n}})). \quad (34)$$

Since the RHS is nonnegative, we are done.

#### D. Compiling the Proof

We are now ready to prove Theorem 1, restated here for convenience.

**Theorem 1.** *Optimal QFI states are exactly those that can be reached from a decoupled, properly ordered state by applying passive transformations within modes having the same  $g_a$ . These optimal QFI states have*

$$H = 2 \sum_{a=1}^N g_a^2 \sinh^2(2r_a). \quad (35)$$

The proof proceeds in two steps. First, we show that the QFI  $H$  satisfies

$$H \leq 2 \sum_{a=1}^N g_a^2 \sinh^2(2r_a). \quad (36)$$

Then we show the bound is saturated for the claimed states.

##### 1. Proving the QFI Upper Bound

We bound the RHS of eq. (10) using that  $\text{Tr}((\mathbf{V}\mathbf{G})^2) \leq \text{Tr}(\mathbf{V}^2\mathbf{G}^2)$ , valid because  $\mathbf{V}$  and  $\mathbf{G}$  are hermitian [18]:

$$H \leq \frac{\text{Tr}(\mathbf{G}^2(\mathbf{V}^2 - \mathbf{I}))}{2}. \quad (37)$$

Equality holds if and only if  $[\mathbf{V}, \mathbf{G}] = 0$ . Next, define

$$\tilde{\mathbf{V}} := \mathbf{V}^2 = \mathbf{K}\mathbf{V}_{\text{in}}^2\mathbf{K}^{-1}. \quad (38)$$

This is a valid covariance matrix for a zero-mean state  $|\tilde{\mathbf{V}}\rangle$  made by passively transforming 1-mode squeezed states with squeezing  $2r_1, 2r_2, \dots, 2r_N$ . Further defining

$$\tilde{\mathbf{V}}_a = \begin{bmatrix} \tilde{V}_{2a-1,2a-1} & \tilde{V}_{2a-1,2a} \\ \tilde{V}_{2a,2a-1} & \tilde{V}_{2a,2a} \end{bmatrix}, \quad (39)$$

we can write eq. (37) as

$$H \leq \frac{1}{2} \sum_{a=1}^N g_a^2 (\text{Tr}(\tilde{\mathbf{V}}_a) - 2). \quad (40)$$

Letting  $\tilde{n}_a$  be the mean photon number in mode  $a$  of  $|\tilde{\mathbf{V}}\rangle$ , recall that  $\text{Tr}(\tilde{\mathbf{V}}_a) - 2 = 4\tilde{n}_a$ . Therefore,

$$H \leq 2 \sum_{a=1}^N g_a^2 \tilde{n}_a. \quad (41)$$

We will have proved eq. (36) if we can show

$$2 \sum_{a=1}^N g_a^2 \tilde{n}_a \leq 2 \sum_{a=1}^N g_a^2 \sinh^2(2r_a). \quad (42)$$

This is where majorization theory enters. Applying Proposition 3 to  $|\tilde{V}\rangle$ , the initial state is described by  $\mathbf{V}_{\text{in}}^2$ , which has squeezing levels  $2r_1, \dots, 2r_N$ , so the initial photon numbers are  $\sinh^2(2\mathbf{r}) = \{\sinh^2(2r_i)\}_{i=1}^N$ . Writing  $\tilde{\mathbf{n}} = \{\tilde{n}_a\}_{a=1}^N$ , the proposition yields

$$\sinh^2(2\mathbf{r}) \succ \tilde{\mathbf{n}}. \quad (43)$$

Finally, recall that we ordered the  $g_a^2$  and  $r_a$  to be nonincreasing, so we can take  $g_a^2 = c_a$  and  $\sinh^2(2\mathbf{r}) = \mathbf{n}$  in Lemma 2, which proves eq. (42) and hence eq. (36).

In summary, we proved our general QFI bound through the following chain of (in)equalities:

$$H = \frac{\text{Tr}((\mathbf{V}\mathbf{G})^2 - \mathbf{G}^2)}{2} \leq 2 \sum_{a=1}^N g_a^2 \tilde{n}_a \leq 2 \sum_{a=1}^N g_a^2 \sinh^2(2r_a). \quad (44)$$

## 2. Optimal QFI States: Saturating the QFI Bound

Having proven the QFI bound eq. (36), we examine when the bound is saturated. We define PODF (properly ordered, damaging-entanglement free) states to be the states claimed to be optimal in Theorem 1. We need to prove that the bound is saturated exactly when the state is PODF.

Consider the first inequality in eq. (44). This inequality is saturated exactly when  $\mathbf{V}$  and  $\mathbf{G}$  commute, i.e. when  $\mathbf{V}$  is block-diagonal with one block for each unique  $g_a$ . In particular, PODF states have this block structure.

Therefore, it remains to show that among the states with this block structure, the PODF states are exactly the ones saturating the second equality in eq. (44). Consider an arbitrary  $\mathbf{V}$  with the block structure, and let the blocks be  $\mathbf{V}_m$ , with  $m$  labeling the blocks. By eq. (23), each of the  $\mathbf{V}_m$  are covariance matrices of pure Gaussian states. Therefore, we can decouple each of the  $\mathbf{V}_m$  using a symplectic orthogonal transformation within each block (by eq. (22)), arriving at the decoupled covariance matrix  $\mathbf{V}_d$ .

Crucially, symplectic orthogonal transformations within each block do not affect  $2 \sum_{a=1}^N g_a^2 \tilde{n}_a$ , since this quantity can be rewritten in terms of  $\text{Tr}(\mathbf{V}_m^2)$  (similar to the RHS of eq. (40)). Thus,  $\mathbf{V}$  is optimal exactly when  $\mathbf{V}_d$  is.

Now, by the discussion around eq. (16) in the main text,  $\mathbf{V}_d$  is optimal if properly ordered. Furthermore, to saturate the second inequality in eq. (44),  $\mathbf{V}_d$  must be properly ordered; otherwise, we can increase  $2 \sum_{a=1}^N g_a^2 \tilde{n}_a$  by switching the 1-mode squeezed states in modes  $a$  and  $b$  that violate proper ordering. Altogether,  $\mathbf{V}$  is optimal exactly when  $\mathbf{V}_d$  is properly ordered, completing the proof of Theorem 1.

Incidentally, notice that  $\mathbf{V}_d$  can be chosen to be diagonal, not just decoupled. In other words, the word “decoupled” in the theorem may be replaced by “diagonal.”

## IV. GENERALIZING TO ARBITRARY PARAMETERIZED PASSIVE TRANSFORMATIONS

So far, we have assumed the modes receive phase shifts of magnitude  $g_a \phi$ , where we want to measure  $\phi$ . We can generalize this to measuring  $\phi$  when the system is acted upon by a parameterized passive transformation  $\mathcal{U}(\phi)$ . In this case, we can write the covariance matrix as

$$\mathbf{V}(\phi) = \mathbf{K}(\phi) \mathbf{V}(0) \mathbf{K}(\phi)^T, \quad (45)$$

where  $\mathbf{K}(\phi)$  is the symplectic orthogonal matrix describing  $\mathcal{U}(\phi)$ . Let us now define the logarithmic derivative

$$\mathbf{g}(\phi) := \mathbf{K}'(\phi) \mathbf{K}(\phi)^{-1}. \quad (46)$$

This is given the letter  $\mathbf{g}$  because we claim it is an element of the Lie algebra of the symplectic orthogonal group. To prove this, note that for any fixed  $\phi_0$ , we have that  $\mathbf{g}(\phi_0)$  is the derivative of  $P(\phi) := \mathbf{K}(\phi) \mathbf{K}(\phi_0)^{-1}$  at  $\phi = \phi_0$ . Moreover,  $P(\phi_0)$  is the identity, and the derivative of a path at the identity is, by definition, an element of the Lie algebra.

Now, since  $\mathbf{g}(\phi)$  is an element of the Lie algebra of the orthogonal group (which contains the Lie algebra of the symplectic orthogonal group), it is anti-symmetric:  $\mathbf{g}(\phi)^T = -\mathbf{g}(\phi)$  (see ref. [19], prop. 3.24, pg. 58). Differentiating eq. (45) and using this anti-symmetry of  $\mathbf{g}(\phi)$ , we have

$$\mathbf{V}'(\phi) = \mathbf{g}(\phi) \mathbf{V}(\phi) + \mathbf{V}(\phi) \mathbf{g}(\phi)^T = [\mathbf{g}(\phi), \mathbf{V}(\phi)]. \quad (47)$$

Comparing with eq. (6), we can't yet rerun the previous derivation because  $\mathbf{g}$  need not be as in eq. (3). We need

**Lemma 3.** Any element  $\mathbf{g}$  in the Lie algebra of the symplectic orthogonal group has the decomposition

$$\mathbf{g} = \tilde{\mathbf{K}}^{-1} \tilde{\mathbf{g}} \tilde{\mathbf{K}}, \quad (48)$$

where  $\tilde{\mathbf{K}}$  is symplectic orthogonal and  $\tilde{\mathbf{g}}$  is in the form of eq. (3).

*Proof.* We use the isomorphism described by eq. (29) between the unitary and symplectic orthogonal groups. Firstly, note that the same formula also gives an isomorphism between the Lie algebras of these groups, which can be seen by differentiating the formula for some path through the identities of the groups. Therefore, associated to  $\mathbf{g}$  is an element  $\mathbf{u}$  in the Lie algebra of the unitary group. This Lie algebra consists of anti-hermitian matrices ([19], prop. 3.24, pg. 58), so  $\mathbf{u}$  may be diagonalized as

$$\mathbf{u} = \mathbf{U}^{-1} \mathbf{D} \mathbf{U}, \quad (49)$$

where  $\mathbf{U}$  is unitary and  $\mathbf{D}$  is diagonal; the diagonal is purely imaginary, so we can write it as  $ig_1, \dots, ig_N$ . Mapping eq. (49) back to the symplectic orthogonal group through eq. (29) yields the lemma.  $\square$

This lemma implies that if we change our basis of modes using the symplectic orthogonal matrix  $\tilde{\mathbf{K}}$  as

$$\mathbf{V} \rightarrow \tilde{\mathbf{K}} \mathbf{V} \tilde{\mathbf{K}}^{-1}, \quad \mathbf{V}' \rightarrow \tilde{\mathbf{K}} \mathbf{V}' \tilde{\mathbf{K}}^{-1}, \quad (50)$$

then we can rewrite eq. (47) as  $\mathbf{V}'(\phi) = [\tilde{\mathbf{g}}(\phi), \mathbf{V}(\phi)]$ . We can now rerun the derivation starting from eq. (3) (except that now,  $H$  will be a function of  $\phi_0$ ).

In summary, we see that for any parameterized unitary, at a given  $\phi = \phi_0$ , we may pick a new set of the modes so that the unitary locally looks like a set of phase shifts on those modes. Accordingly, the QFI at  $\phi_0$  will be damaged by entanglement between these new modes. Note that these new modes will generally no longer correspond to individual paths. Thus, the trade-off involves entanglement between modes rather than paths in this general case.

- 
- [1] C. Weedbrook, S. Pirandola, R. García-Patrón, N. J. Cerf, T. C. Ralph, J. H. Shapiro, and S. Lloyd, Reviews of Modern Physics **84**, 621 (2012).
  - [2] R. Simon, N. Mukunda, and B. Dutta, Phys. Rev. A **49**, 1567 (1994).
  - [3] A. Monras, arXiv preprint arXiv:1303.3682 (2013).
  - [4] O. Pinel, J. Fade, D. Braun, P. Jian, N. Treps, and C. Fabre, Ultimate sensitivity of precision measurements with gaussian quantum light : a multi-modal approach (2011), arXiv:1105.2644 [quant-ph].
  - [5] T. Matsubara, P. Facchi, V. Giovannetti, and K. Yuasa, New Journal of Physics **21**, 033014 (2019).
  - [6] A. S. Holevo and R. F. Werner, Phys. Rev. A **63**, 032312 (2001).
  - [7] One might also consider a scenario in which  $g_1, \dots, g_n$  are 1 and  $g_m = 0$  for  $m > n$ ; this would appear to be naturally bipartite between the first  $i$  modes and the rest of the system. We leave it the future work as to whether a simple formula for the QFI in terms of an entanglement measure also exists in this case.
  - [8] R. Simon, S. Chaturvedi, and V. Srinivasan, Journal of Mathematical Physics **40**, 3632 (1999).
  - [9] A. Serafini, F. Illuminati, and S. De Siena, Journal of Physics B: Atomic, Molecular and Optical Physics **37**, L21 (2003).
  - [10] Arvind, B. Dutta, N. Mukunda, and R. Simon, Pramana **45**, 471 (1995).
  - [11] M. Nielsen and I. Chuang, Cambridge, England (2000).
  - [12] B. C. Arnold, Majorization and the Lorenz order: A brief introduction, Vol. 43 (Springer Science & Business Media, 2012).
  - [13] A. W. Marshall, I. Olkin, and B. C. Arnold, Inequalities: theory of majorization and its applications (Springer, 1979).
  - [14] E. Chitambar and G. Gour, Reviews of Modern Physics **91**, 10.1103/revmodphys.91.025001 (2019).
  - [15] J. Eisert, S. Scheel, and M. B. Plenio, Phys. Rev. Lett. **89**, 137903 (2002).
  - [16] J. Fiurášek, Phys. Rev. Lett. **89**, 137904 (2002).
  - [17] G. Giedke and J. Ignacio Cirac, Phys. Rev. A **66**, 032316 (2002).
  - [18] There are several ways of proving this inequality. One way, suggested by [5], is to realize that it is equivalent to  $\text{Tr} \left( (i(\mathbf{V}\mathbf{G} - \mathbf{P}\mathbf{V}))^2 \right) \geq 0$ . And this latter inequality is true because  $i(\mathbf{V}\mathbf{G} - \mathbf{P}\mathbf{V})$  is hermitian. Equality holds exactly when this operator is zero.
  - [19] B. C. Hall, Lie groups, Lie algebras, and representations (Springer, 2013).
